# Supplementary material for: Transient absorption and photocurrent microscopy show hot electron supercollisions describe the rate-limiting relaxation step in graphene
Source: arXiv:1310.6428 source file (2013-10-23)
Supplement: Supplementary file 1 [file supplement_McEeun.pdf]

# **Supplement:** *Transient absorption and photocurrent microscopy show hot electron supercollisions describe the rate-limiting relaxation step in graphene*

Matt W. Graham[1,2], Su-Fei Shi[1,2], Zenghui Wang[1,3], Daniel C. Ralph[1,2], Jiwoong Park[1,3], Paul L. McEuen[1,2]

1. Kavli Institute at Cornell for Nanoscale Science, Ithaca, NY 14853, USA
2. Laboratory for Atomic and Solid State Physics, Cornell University
3. Department of Chemistry and Chemical Biology, Cornell University

## S.1: Fabrication of CVD Suspended Graphene and Graphene *p-n* junctions

### S1.1 Suspended graphene

Devices with suspended graphene stripes are fabricated by transferring pre-patterned CVD-grown graphene on to pre-fabricated device structures with patterned microtrenches.

The CVD graphene is grown on Alfa Aesar 0.025mm, 99.8% pure copper foils. The as-grown graphene covered copper piece is then spin-coated with photoresist (MICROPOSIT S1813). Arrays of stripes with different widths are then patterned onto the copper piece using photolithography. The graphene in the exposed area is then removed with oxygen plasma. After stripping the remaining photoresist, the copper piece with the patterned graphene stripes is coated with a thin layer (~50 nm) of PMMA and put into copper etch (CE-200).

After all the cupper substrate is dissolved, the remaining PMMA/graphene floats are transferred into 6 baths of DI water to clean the graphene. The floats are then transferred onto the pre-fabricated substrates with the graphene stripes roughly aligned perpendicular to the microtrenches. After the PMMA piece completely dries and conforms to the substrate surface, the sample is placed in anisole followed by acetone to dissolve the PMMA layer. Finally, the devices are dried using a critical point dryer (Tousimis Automegasamdri-915B) to preserve the suspended graphene stripes across the microtrenches. Images of a typical resulting device are shown in Fig. 5b insets of the main text.

### S.1.2 Graphene *p-n* junctions

Micro-Raman was used to confirm the growth of large-grain single-layer graphene with no visible D peak, indicative of high quality growth. Graphene was transferred using the lift-off technique onto a 300 nm $SiO_2$ layer grown on top of a silicon wafer which serves as the global back-gate (BG). The large-grain growth graphene is divided into 30 × 50 μm stripes using photolithography followed by oxygen plasma etching. Electrode pads of titanium/gold (3 nm/150 nm) are deposited along graphene stripes with variable source-drain distances of 10 or 20 μm. A good dielectric separation with the top gate is achieved with 10 nm of $SiO_2$ by electron beam deposition, followed by $HfO_2$ atomic layer deposition. Finally, an optically translucent top gate of titanium/gold (2 nm/20 nm) is deposited along the center of the source-drain gap with a width of 6 μm. The device is mounted in an Oxford HI-RES liquid helium cryostat. The CVD graphene photodetector device had a characteristic high mobility of ~8,000 $cm^2V^{-1}s^{-1}$ with centrally located Dirac points in conductance sweeps.

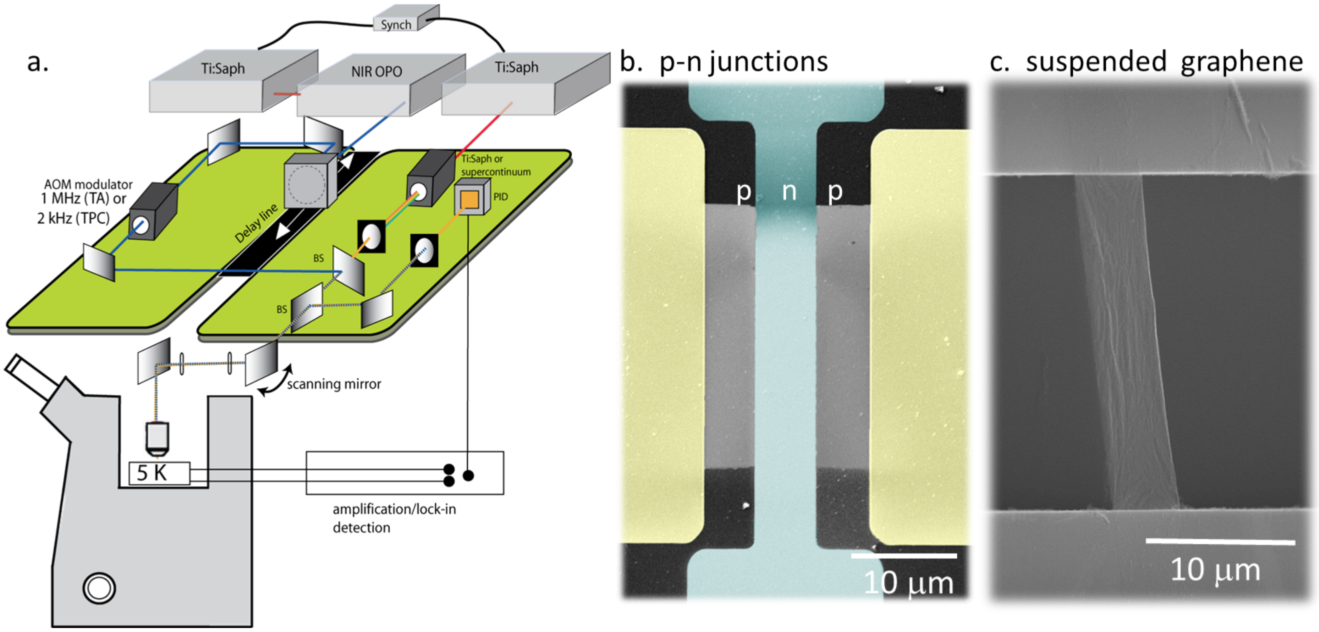


Figure S1: **(a)** Overview of experimental setup for simultaneous transient photocurrent and absorption measurements. The light sources are either a Ti:Saph Mira 900 pump, supercontinuum generation probe, or a Ti:Saph Mira 900 pump and a synchronously locked (Coherent SL-AP) NIR/MIR probe generated by an APE optical parametric oscillator (OPO) **(b)** SEM image of single layer graphene. Current is collected at the source-drain contacts (gold, false color). The graphene sheet is capacitively coupled to the global back gate and local top gate (aqua). **(c)** SEM of a trench-suspended graphene segment.

## S.2: Transient Optical Conductivity

In transient absorption, we measure the change in the amplitude of reflected probe-beam light at an energy $E_o$, in the presence ($R_2$) and absence ($R_1$) of a pump beam. Assuming optical excitation conditions, transient reflectivity is related to the optical conductivity by[7]:

$$\frac{\Delta R(t, E_o)}{R} = \frac{R_2 - R_1}{R_1} = \frac{4}{n_s^2 - 1}\frac{4\pi}{c}\sum_i \mathrm{Re}\left[\sigma_i\left(E_o, T_e(t)\right) - \sigma_i\left(E_o, T_l\right)\right]$$

To satisfactorily fit our TA data we require a minimum of two components. The first timescale ($\tau_1$) contains multiple fast processes beyond our temporal resolution such as electron thermalization and optic phonon emission. The application of the SC-model to the second timescale ($\tau_2$), is the focus of this paper. Both interband and intraband can contribute to the total optical conductivity, $\sigma_{TOT} = \sigma_{inter} + \sigma_{intra}$. When the Fermi population are evaluated (to first order) one obtains[7]:

$$\frac{\Delta R(t)_{inter}}{R} \propto \tanh\left(\frac{E_o \pm E_F}{2k_B T_e(t)}\right) - \tanh\left(\frac{E_o \pm E_F}{2k_B T_l}\right) \qquad \text{(S1)}$$

$$\frac{\Delta R(t)_{intra}}{R} \propto \frac{\Gamma k_B T_e(t)}{(E_o \pm E_F)^2 + \Gamma^2} - \frac{\Gamma k_B T_l}{(E_o \pm E_F)^2 + \Gamma^2} \qquad \text{(S2)}$$

Here, the absolute sign of the intraband and interband transient contribution are opposite, permitting easy experimental separation.[7] By varying $E_o$, we show in Fig. S2a that the interband contribution to the optical conductivity dominates for the NIR probe energies used in the manuscript. Consequently, this paper ignores the interband contribution. The transient intraband contributions are investigated in depth elsewhere.[7]

## S.3: Pump and Probe Power dependence

The electronic heat capacity for doped graphene, $C_e = \alpha T_e$, suggests that for a photon flux $F_{\mathbf{in}}$ that the initial temperature

is $T_o \propto \sqrt{2F_{\mathbf{in}}/\alpha}$.[6] Accodingly, evaluating the transient optical response in Eq. S3 at the $t$=0 conditions predicts,

$$\frac{\Delta R\left(F_{\mathbf{in}}\right)_{inter}}{R} \propto \tanh\left(\frac{E_o - E_F}{2k_B\sqrt{2F_{\mathbf{in}}/\alpha}}\right) - \tanh\left(\frac{E_o - E_F}{2k_BT_l}\right) \qquad \text{(S3)}$$

Using Eq. S3 to fit (red lines) the suspended graphene data in Fig. S2b, we show the pump-amplitude dependence is well captured by the above form. In contrast, we show the pump scales linearly with the probe power; as predicted by a genernalized heterodyne pump-probe response.

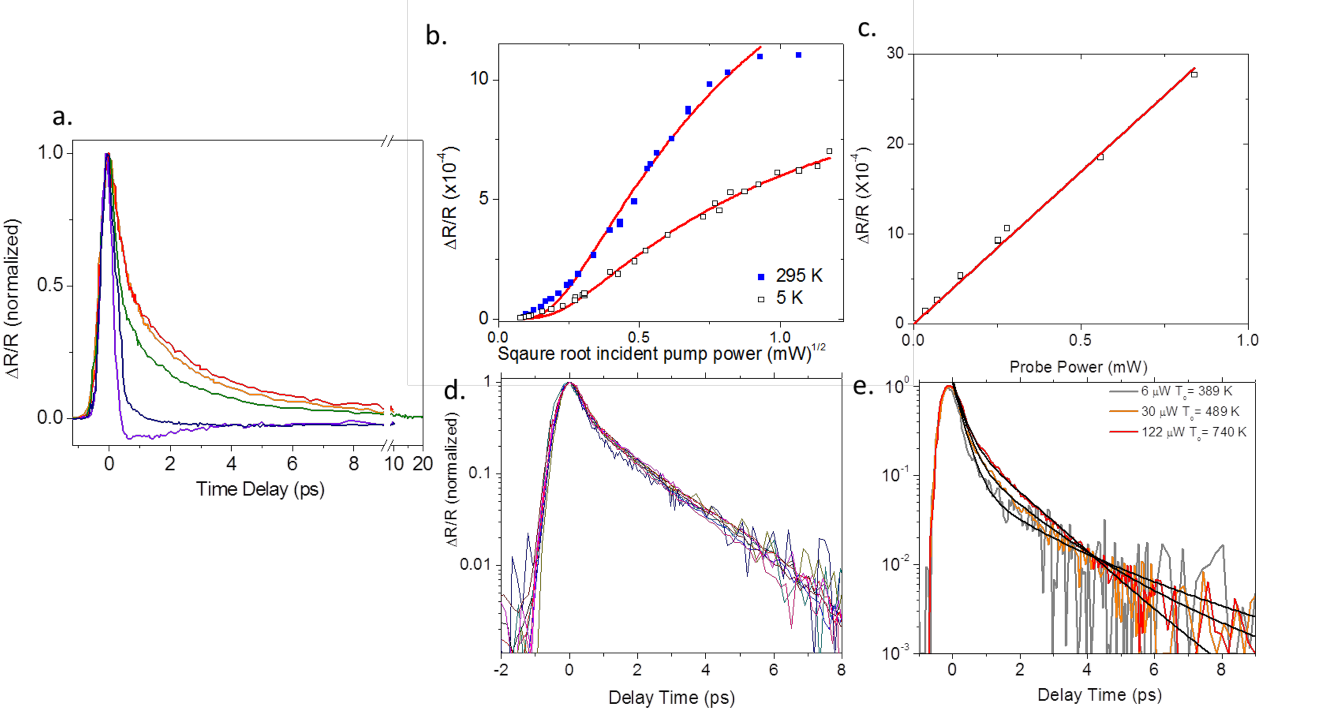


**Figure S2: (a)** Scanning the probe energy from 0.74 eV (red) to 1.32 eV (navy), suspended graphene at 5 K shows a transition toward intraband dominated kinetics. **(b)** Transient amplitude at $t$=0.1 ps vs. square root of incident laser pump power. Red lines are fits to Eq. S5 at 295 and 5 K. **(c)** The transient absorption signal depends linearly on the applied probe power. **(d)** At $T_l$=5 K, the transient decay dynamics are independent of pump fluence when normalized. **(e)** Conversely, at $T_l$= 295K, the kinetic decay depends weakly on applied pump power. Using the SC model we can predict the dependence by adjusting the initial electron temperature to fit the data (black lines).

## S.4: Lattice Temperature Dependence

After the electrons/holes thermalize, the optical conductivity can be described by a hot electron (or hole) temperature. In the hot phonon (HP) temperature model, the hot electron temperature decays approximately inversely with time according to the temperature of the hot optical phonon bath. We assume the hot phonon population, $p(t)$ decays exponentially from an initial temperature, $T_{op}$ with a lifetime $\tau_{ph}$ , i.e.

$$p(t) = \frac{P}{1+\exp\left(\hbar\omega_{op}/k_BT_{op}(t)\right)} \approx P\exp\left(-\frac{\hbar\omega_{op}}{k_BT_{op}} - \frac{t}{\tau_{ph}}\right)$$

In the hot phonon model, $T_{op}(t) \approx T_e(t)$, which gives:

$$\frac{\hbar\omega_{op}}{k_BT_e(t)} = \frac{\hbar\omega_{op}}{k_BT_{op}} + \frac{t}{\tau_{ph}} \quad OR \quad T_e(t) = \frac{T_o}{1+k_BT_{op}\,t/\left(\tau_{ph}\hbar\omega_{op}\right)}$$

The resulting hot electron temperature is then approximately independent of the lattice temperature (except for substrate heating contributions which are expected to be small at our probe energies given the relative graphene Debye temperature).

Alternatively, using the SC model[4] for doped graphene one obtains a different lattice temperature dependence:

$$\frac{dT_e(t)}{dt} = -\frac{A}{\alpha}\frac{T_e(t)^3 - T_l^3}{T_e(t)} \qquad \text{(S3).}$$

In Fig. S3, we analytically solve the above differential equation for a given lattice temperature. The initial condition must take into account both the electronic energy deposited by the laser pulse, and the existing energy in the lattice. The initial, thermalized temperature can be approximated as $T(0) = T_o = \sqrt{T_{eo}^2 + T_l^2}$. In Fig. S3, the SC predicts a strong lattice temperature dependent trend that reverses direction when the probe energy, $E_o <\sim 0.15$ eV.

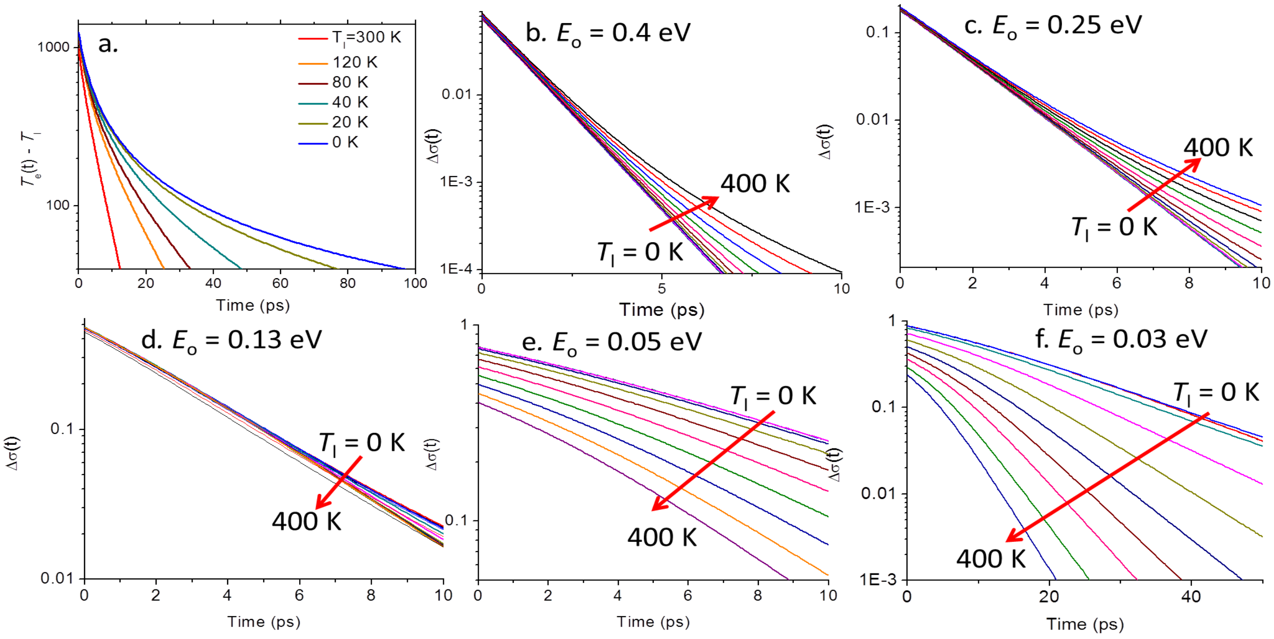


**Figure S3: (a)** Analytic solutions for the the SC-controlled electron temperature for a rate coefficient of $2.5 \times 10^{-4} K^{-1} ps^{-1}$. **(b-f)** The predicted transient interband response of the SC contribution to the kinetics. At high probe energies, the TA decay becomes moderately slower for low lattice temperatures, conversely for probe energies near the Fermi energy predicted decay becomes markedly longer. This can be understood by comparing Figures S3a and 3c (*inset*).

## S.5: Fermi level dependence:

When $T_e(t) >> T_l$ the SC model can be approximated as $T_e(t) = T_o / \left(1 + AT_o t/\alpha\right)$, which has the same functional form as the HP model presented above. Inserting into Eq. S1, the SC interband transient reflectivity contribution becomes,

$$\frac{\Delta R(t)_{inter}}{R} \propto \tanh\left(\frac{E_o \pm E_F}{2k_B T_o}\right)\tanh\left(\frac{At}{\alpha}\frac{E_o \pm E_F}{2k_B}\right) - \tanh\left(\frac{E_o \pm E_F}{2k_B T_l}\right) \qquad \text{(S4)}$$

This predicts an approximately exponential decay with an effective liftetime: $\tau_2^{-1} = A/k_B\alpha\left(E_o - E_F\right)$. In this paper the intrinsic graphene doping was determined by plotting the approximate decay rate, $\tau_2^{-1}$ vs. $E_o$ (see Fig. 5). The gate induced doping was determined using the capacitance between the applied back gate voltages and the graphene sheet.

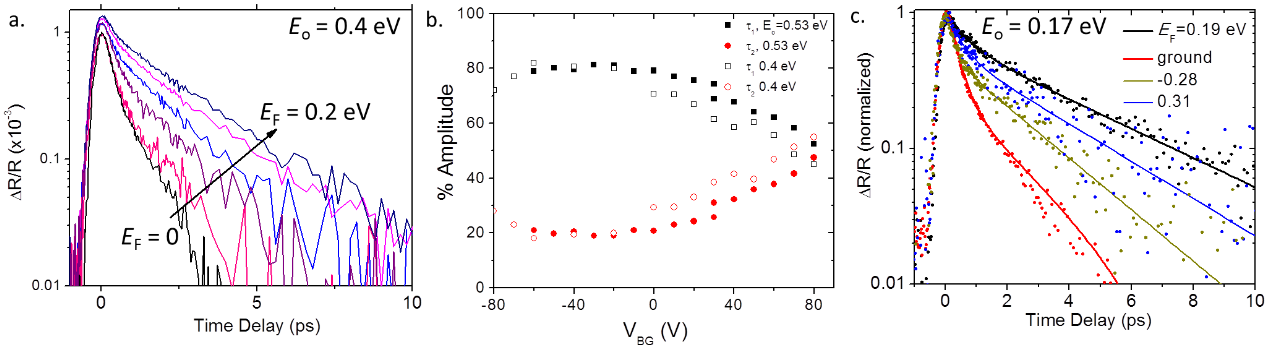

**Fig S4**: **(a)** The decay rates of the $T_l$ = 10 K transient absorption for 1.25 eV pump, 0.8 eV probe vary markedly as a function of back gate, corresponding with the Fermi level indicated. **(b)** As a function of back gate (Fermi energy) we show the percent amplitude of the $\tau_2$ component grows from ~20% to 60% weight. **(c)** The decay rates and amplitudes of the $T_l$ = 10 K transient absorption for $E_0$=0.17 eV mid-IR probe vary markedly as a function of back gate, corresponding with the Fermi level indicated.

## S.6: Transient Photocurrent Response Function

Please see ref. 6 and its supplemental section for details on the transient photocurrent response function.

## S.7: References


[1] N. M. Gabor, J. C. W. Song, Q. Ma, N. L. Nair, T. Taychatanapat, K. Watanabe, T. Taniguchi, L. S. Levitov, and P. Jarillo-Herrero, Science, 2011, 334(6056), 648 –652.

[2] J. C. Song, M. S. Rudner, C. M. Marcus, and L. S. Levitov, Nano Lett, 2011, 11(11), 4688-4692.

[3] M. Breusing, C. Ropers, and T. Elsaesser, Phys Rev Lett, 2009, 102(8), 086809.

[4] J. C. W. Song, M. Y. Reizer, and L. S. Levitov, arXiv:1111.4678, 2011.

[5] J. C. W Song and L. S Levitov arXiv:1112.5654 [cond-mat.mes-hall].

[6] M.W. Graham, S. Shi, D. Ralph, J. Park, P.L. McEuen, Nature Physics, 9, 103, 2013

[7] L. Malard. K.-F. Mak, A. Castro, N. Peres, and T.F. Heinz, *New Journal of Physics*, 2013, 15, 015009
